# Supplementary material for: Generalized Relative Neighborhood Graph (GRNG) for Similarity Search
Source: arXiv:2208.10022 source file (2022-08-22)
Supplement: Supplementary file 1 [file fig_supplementary_GRNG_RNG_Fixed_N_Results.tex]

\begin{figure}[h!]
    \centering
    % %add desired spacing between images, e. g. ~, \quad, \qquad, \hfill etc. 
    % (or a blank line to force the subfigure onto a new line)
    \begin{minipage}{0.45\textwidth}
        \includegraphics[width=\textwidth]{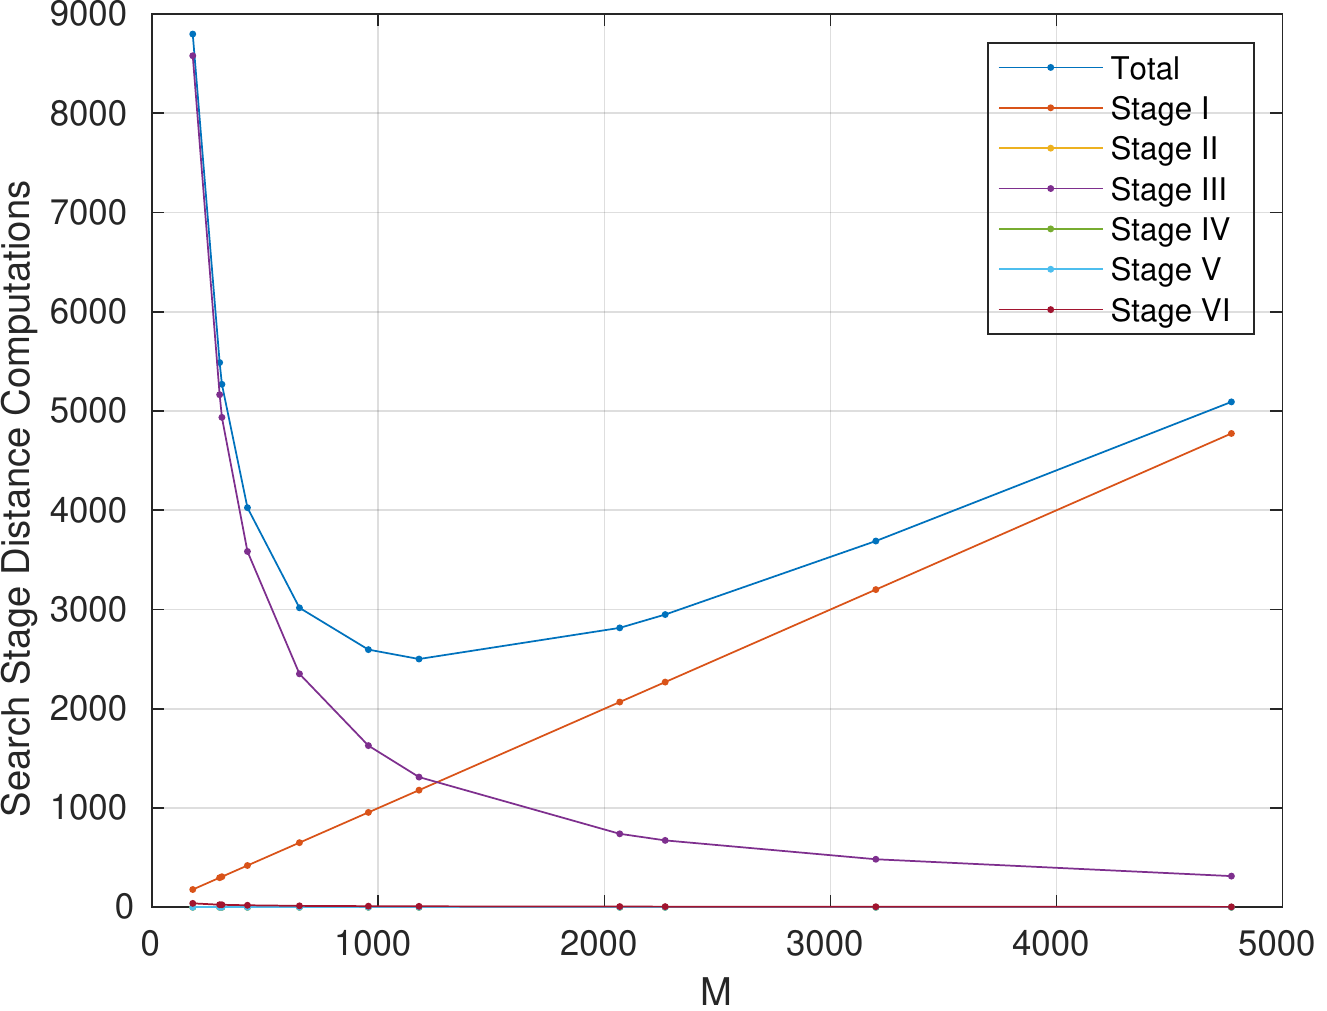}
    \end{minipage}
    \begin{minipage}{0.45\textwidth}
        \includegraphics[width=\textwidth]{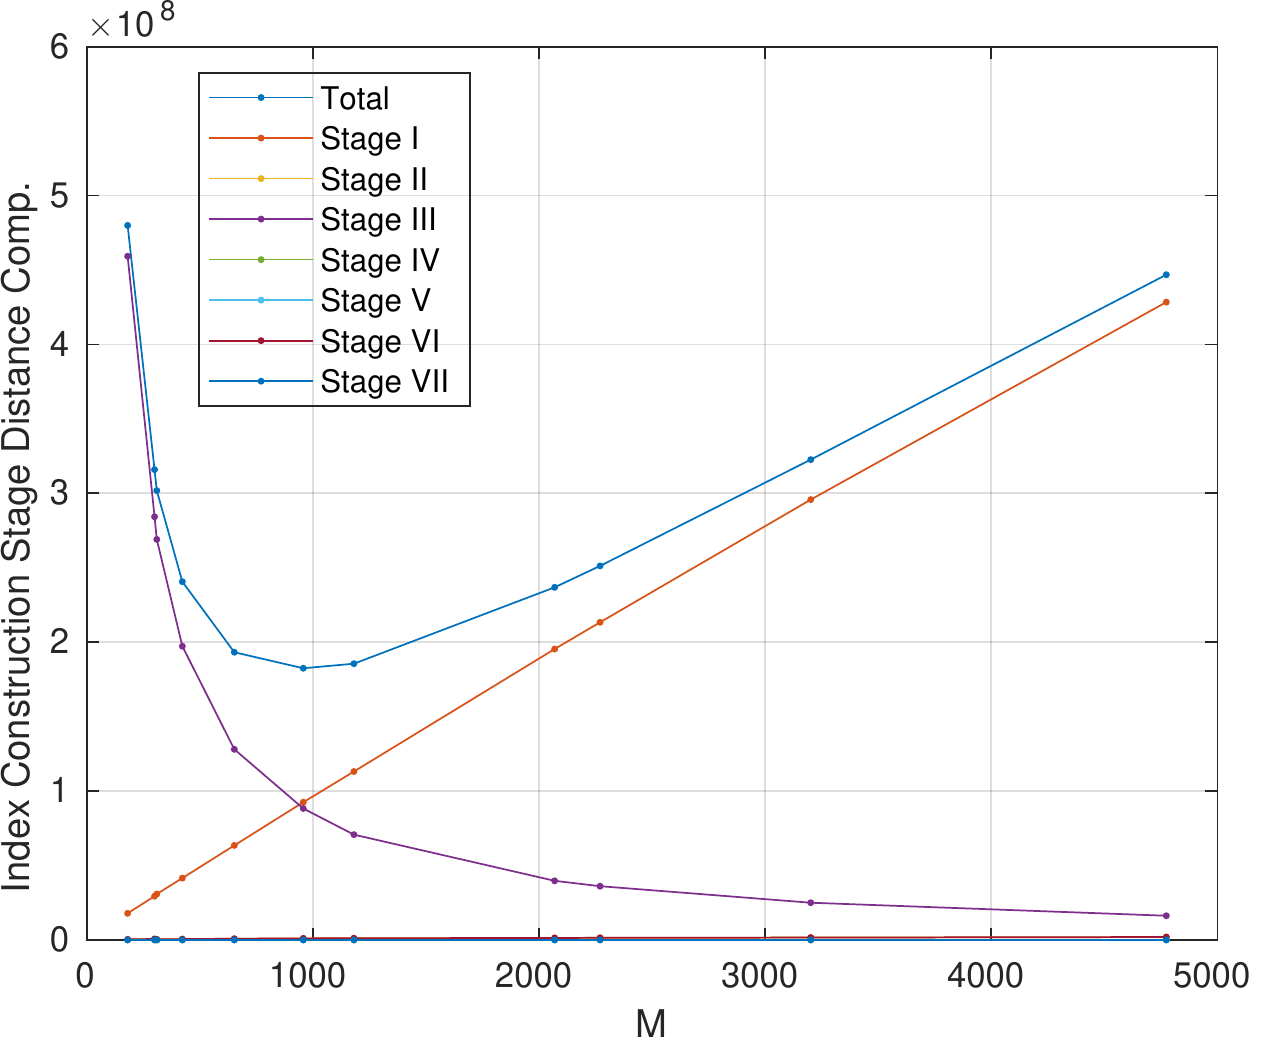}
    \end{minipage}

    \begin{minipage}{0.45\textwidth}
        \includegraphics[width=\textwidth]{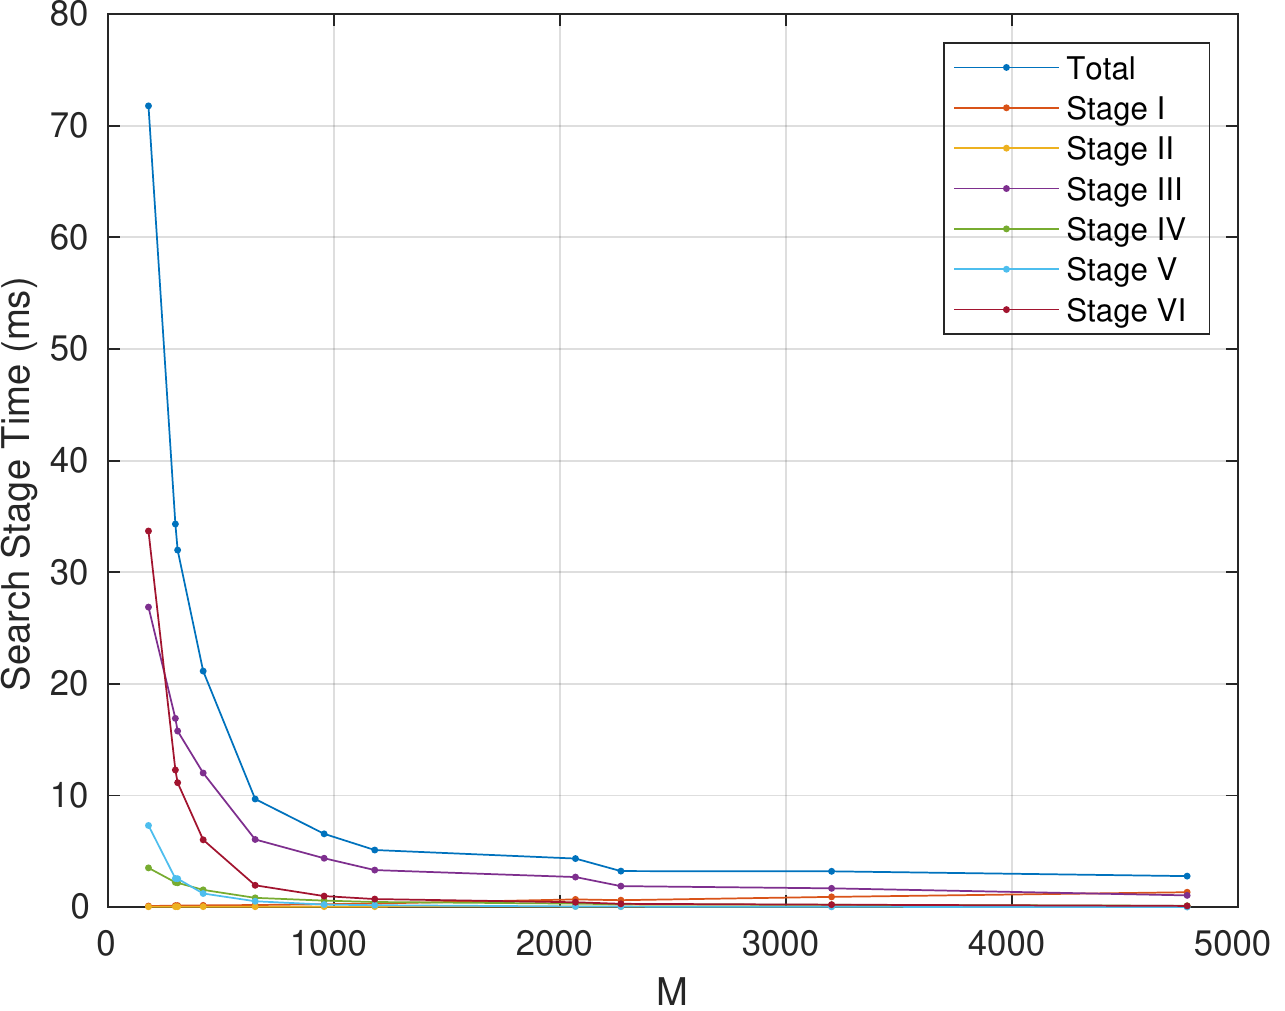}
    \end{minipage}
    \begin{minipage}{0.45\textwidth}
        \includegraphics[width=\textwidth]{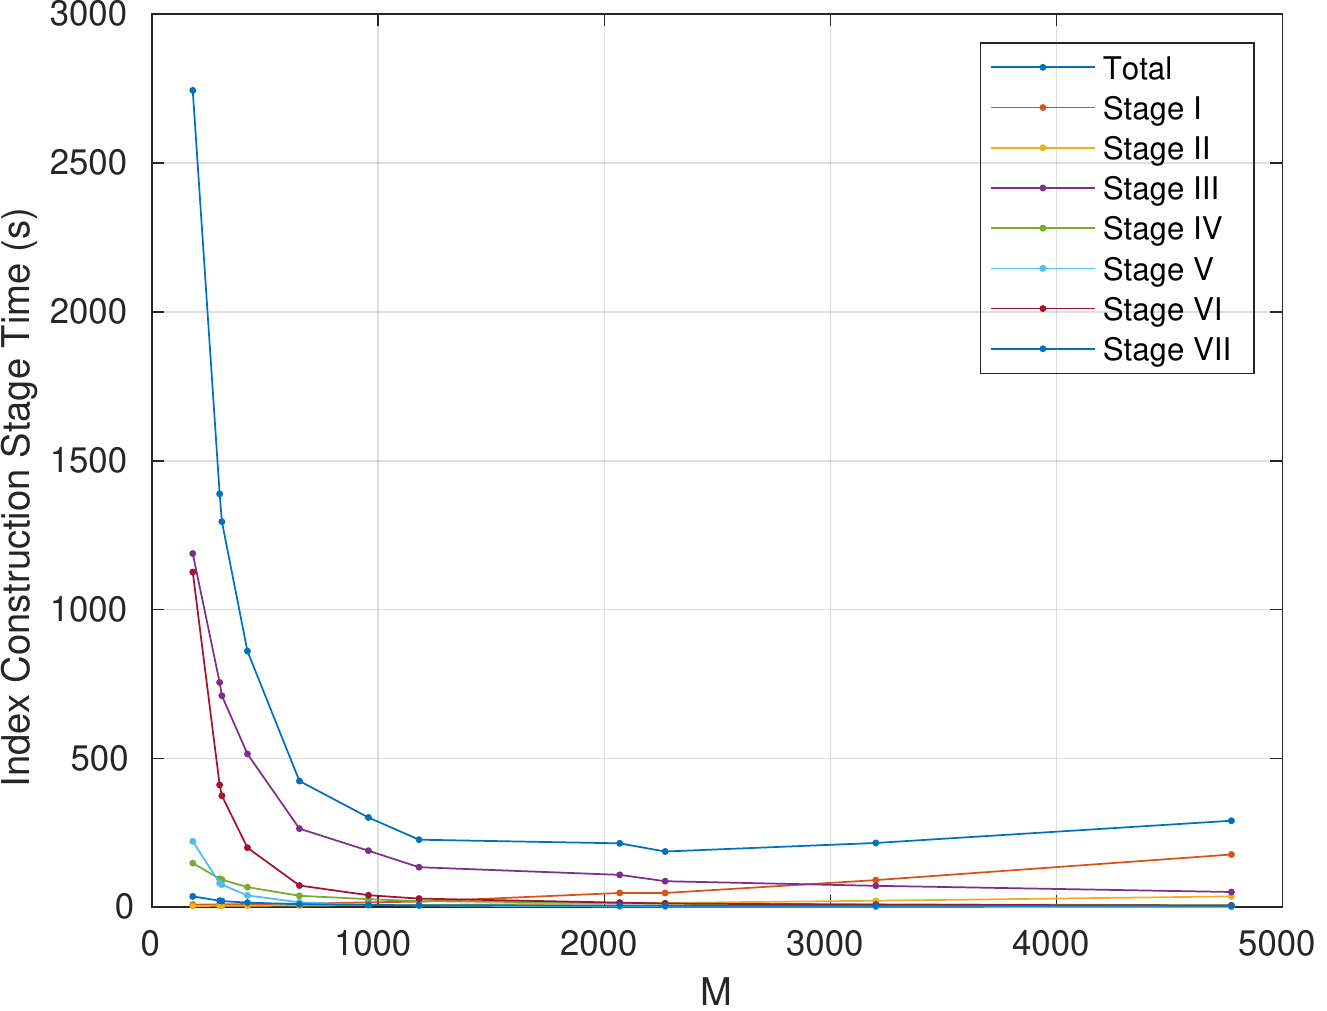}
    \end{minipage}
    
    \begin{minipage}{0.31\textwidth}
        \includegraphics[width=\textwidth]{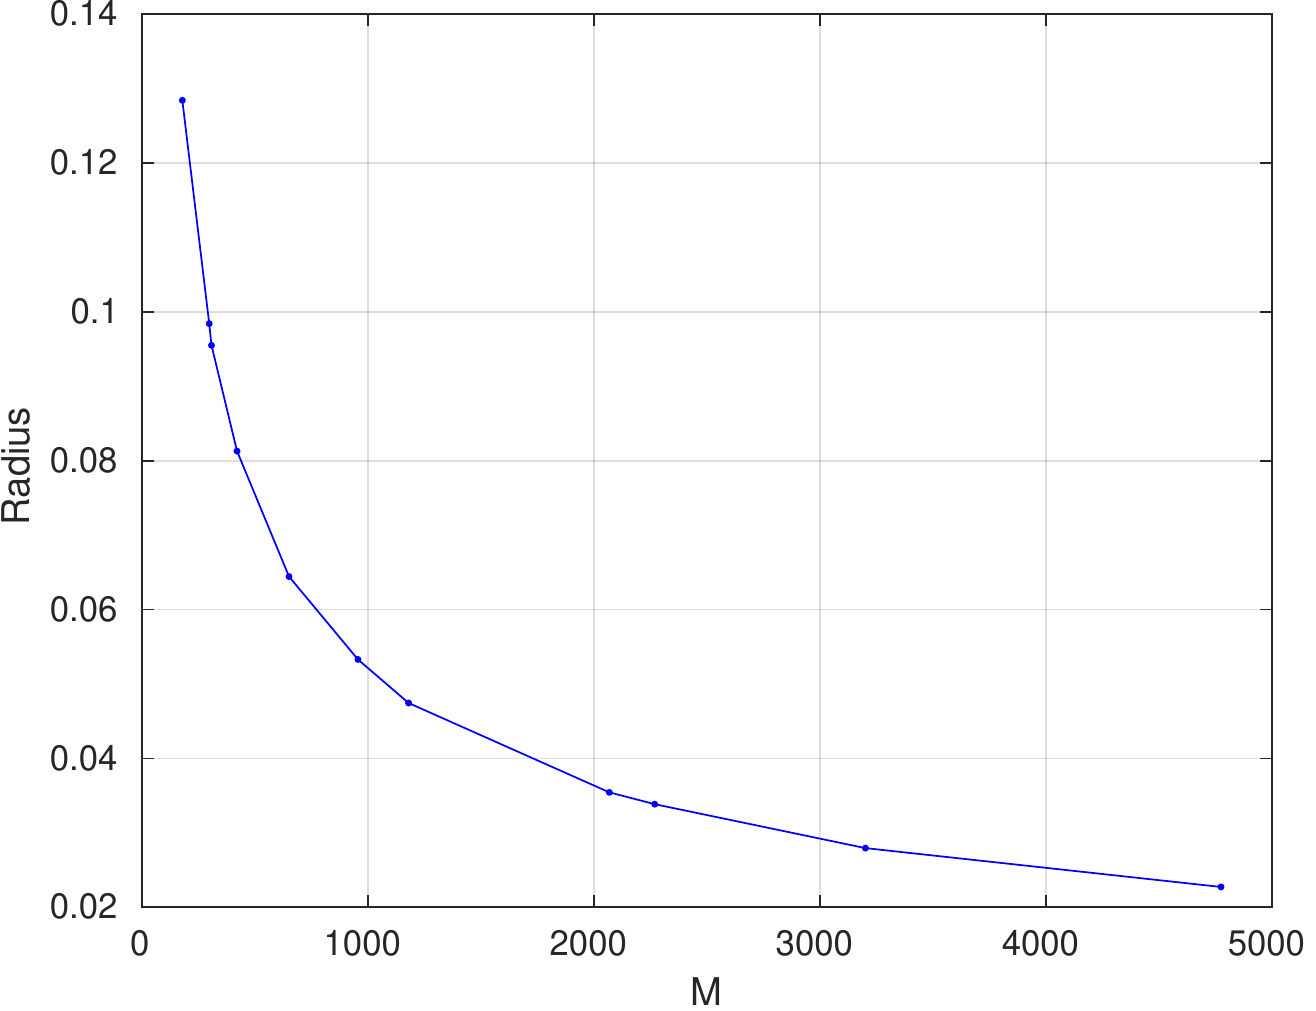}
    \end{minipage}
    \begin{minipage}{0.31\textwidth}
        \includegraphics[width=\textwidth]{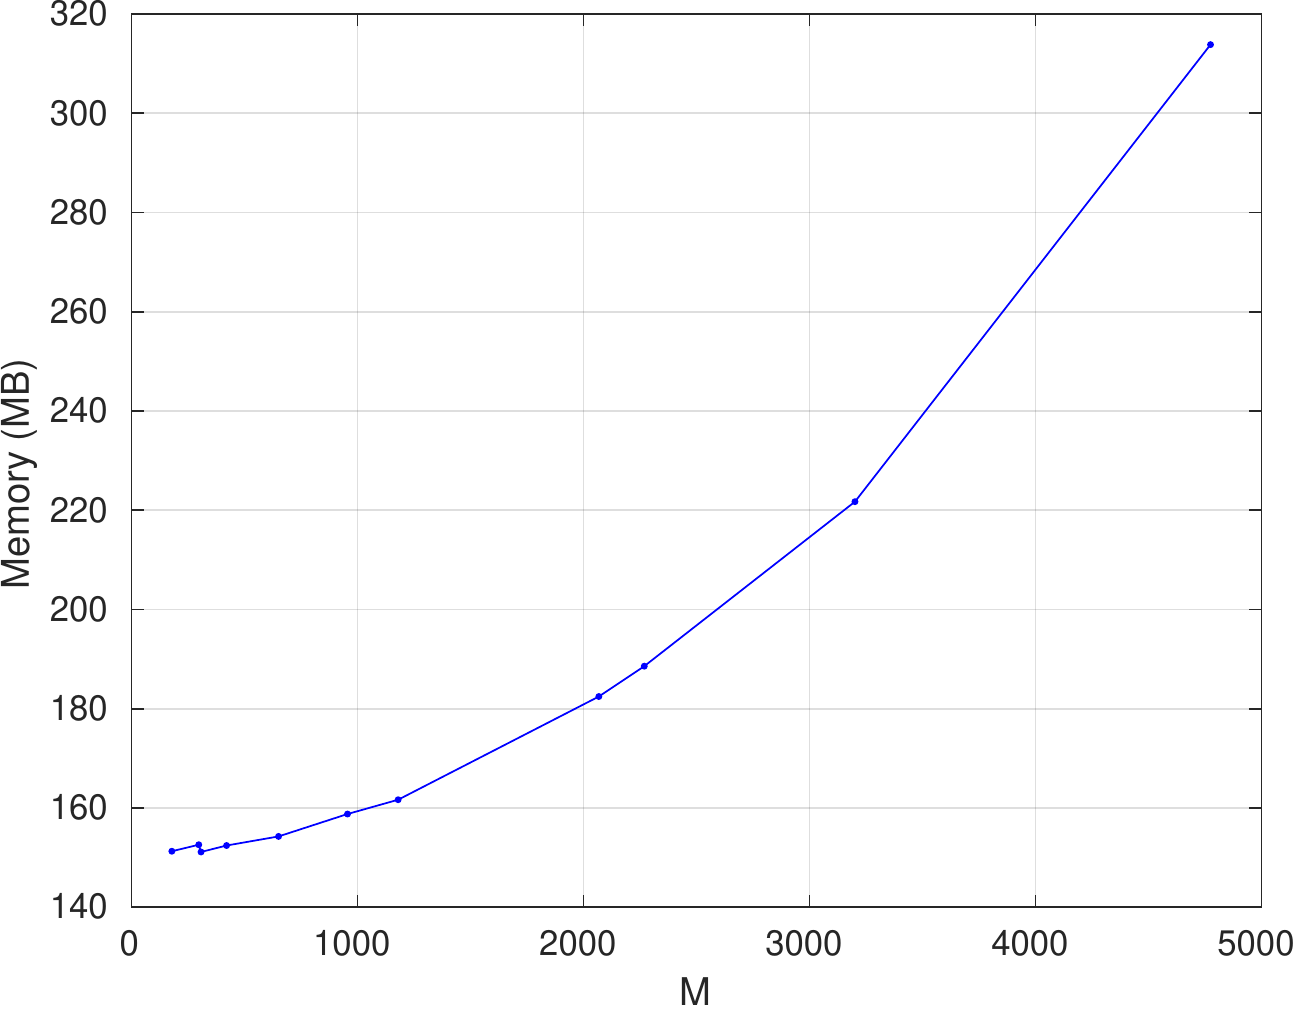}
    \end{minipage}
    \begin{minipage}{0.31\textwidth}
        \includegraphics[width=\textwidth]{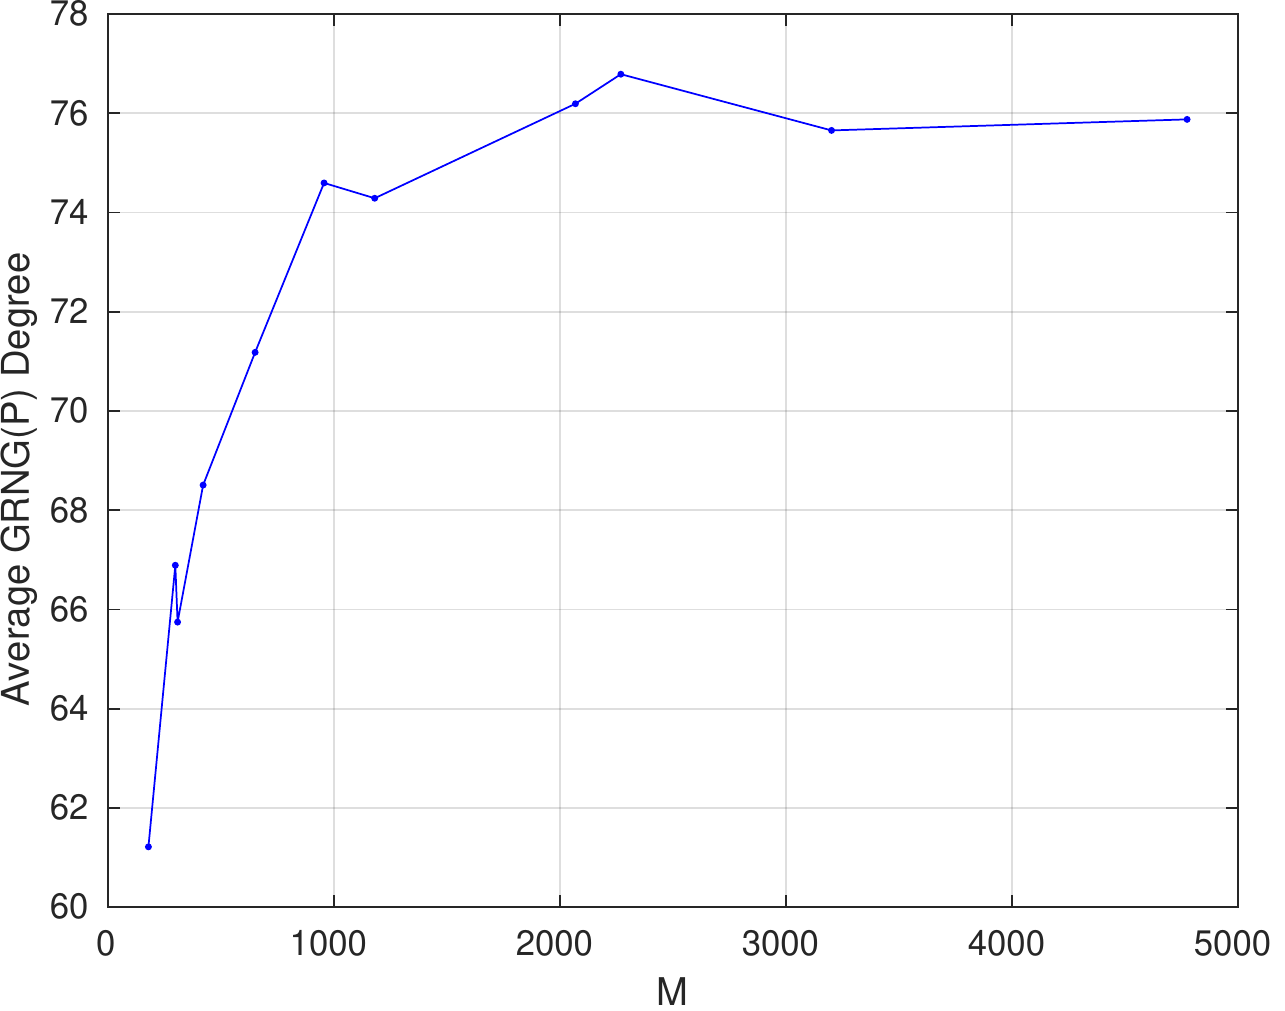}
    \end{minipage}
    
    \caption{\footnotesize Statistics for the optimization of a 2-Layer GRNG-RNG hierarchy with a fixed $N=102,400$ on 2D, uniformly distributed data.}
    \label{fig:supplementary_GRNG_RNG_Fixed_N_Results}
\end{figure}
