# Supplementary material for: Generalized Relative Neighborhood Graph (GRNG) for Similarity Search
Source: arXiv:2208.10022 source file (2022-08-22)
Supplement: Supplementary file 2 [file supplementary.tex]

%\section{Supplementary Material}

%******************************************************
%------------------------------------------------------
% FIG:10, Generalized Lune Examples
%
% \vspace{-0.5cm}
\input{assets/figures/luneVariationExamples/fig:luneVariationExamples}

\input{assets/figures/2L_GRNG_RNG_Results/fig:supplementary_GRNG_RNG_Fixed_N_Results}

\input{assets/tables/results_uniform/results_grng_rng/table:grng_rng_main}

\input{assets/tables/results_uniform/results_grng_grng_rng/table:grng_grng_rng_main}

\input{assets/tables/results_uniform/results_grng_hierarchies/table:results_grng_hierarchies_main}

% do this as a figure instead
%\input{assets/tables/results_uniform/results_grng_hierarchies/table_results_grng_hierarchies_layers}
